# Supplementary material for: [CII] halos in ALPINE galaxies: smoking-gun of galactic outflows?
Source: arXiv:2212.08083 source file (2022-12-15)
Supplement: Supplementary file 1 [file additional_def.tex]

\let\oldnabla\nabla
\renewcommand{\nabla}{\vec{\oldnabla}}
