# Supplementary material for: [CII] halos in ALPINE galaxies: smoking-gun of galactic outflows?
Source: arXiv:2212.08083 source file (2022-12-15)
Supplement: Supplementary file 2 [file definitions.tex]

%%%%% AUTHORS - PLACE YOUR OWN COMMANDS HERE %%%%%

% Please keep new commands to a minimum, and use \newcommand not \def to avoid
% overwriting existing commands. Example:
%\newcommand{\pcm}{\,cm$^{-2}$}	% per cm-squared

% quick alias
\def\be{\begin{equation}}
\def\ee{\end{equation}}

\def\gsim{\lower.5ex\hbox{\gtsima}} 
\def\lsim{\lower.5ex\hbox{\ltsima}} 
\def\gtsima{$\; \buildrel > \over \sim \;$} 
\def\ltsima{$\; \buildrel < \over \sim \;$} \def\gsim{\lower.5ex\hbox{\gtsima}} 
\def\lsim{\lower.5ex\hbox{\ltsima}} 
\def\simgt{\lower.5ex\hbox{\gtsima}} 
\def\simlt{\lower.5ex\hbox{\ltsima}}

% solar stuff units

% units

% quantities defs

% additional wrappers for quantities and units

% LINES
\def\S*{$\Sigma_{\rm SFR}$}

%\def\CII{[CII]~} 
%\def\CIII{CIII]~}
% IONS

% ion variables

% MIX

% COLORS

\definecolor{apcolor}{HTML}{b3003b}
\definecolor{afcolor}{HTML}{800080}
\definecolor{lvcolor}{HTML}{DF7401}
\definecolor{mdcolor}{HTML}{01abdf} %mahsa and davide
\definecolor{cbcolor}{HTML}{ff0000}
\definecolor{sccolor}{HTML}{cc5500} %stefano
\definecolor{sgcolor}{HTML}{00cc7a}
