# Supplementary material for: [CII] halos in ALPINE galaxies: smoking-gun of galactic outflows?
Source: arXiv:2212.08083 source file (2022-12-15)
Supplement: Supplementary file 3 [file pack.tex]

% MNRAS is set in Times font. If you don't have this installed (most LaTeX
% installations will be fine) or prefer the old Computer Modern fonts, comment
% out the following line
\usepackage{newtxtext,newtxmath}
% Depending on your LaTeX fonts installation, you might get better results with one of these:
%\usepackage{mathptmx}
%\usepackage{txfonts}

% Use vector fonts, so it zooms properly in on-screen viewing software
% Don't change these lines unless you know what you are doing
\usepackage[T1]{fontenc}
\usepackage{ae,aecompl}

%%%%% AUTHORS - PLACE YOUR OWN PACKAGES HERE %%%%%

% Only include extra packages if you really need them. Common packages are:
\usepackage{graphicx}	% Including figure files

         % remove conflict for dual definition
\usepackage{amsmath}	% Advanced maths commands
\usepackage{amssymb}	% Extra maths symbols
\usepackage{comment}
\usepackage{siunitx}
\usepackage{booktabs}

\usepackage{xcolor}
